# Supplementary material for: Not All Relations are Equal: Mining Informative Labels for Scene Graph Generation
Source: arXiv:2111.13517 source file (2022-04-04)
Supplement: Supplementary file 1 [file supp.tex]

\section{Appendix}

\section{Meeting Notes}

\noindent
\textbf{Oct 14, 2021 - Meeting with Hakan and Basura}

\begin{itemize}
    \item Try logit adjustment only with implicit labels frequency
    \item Some qualitative analysis for logit adjustment
    \item Basura suggested to predict pseudo-labels using distance between represnetations aas per this paper - \url{https://openaccess.thecvf.com/content/ICCV2021/papers/Assran_Semi-Supervised_Learning_of_Visual_Features_by_Non-Parametrically_Predicting_View_Assignments_ICCV_2021_paper.pdf}
    (maybe try this in next iteration)
    \item instead of confidence thresholding use some other measure such as diversity/entropy/logit ratio to choose pseudo-labels
    \item Different mixup strategies such as mixing only labels that have some correlations (this might require knowledge of the matrix annotations). 
    \item Arushi Stuff to do
        \begin{itemize}
            \item Write method for what is already there
            \item clean up tables and shortlist what to put finally
            \item do image retrieval experiments (urgent)

        \end{itemize}
\end{itemize}

\noindent
\textbf{Oct 7, 2021 - Meeting with Hakan}

\begin{itemize}
    \item For confidence thresholding, look at \textbf{logits} that might give a better separation as compared to after softmax. 
    \item Maybe try dynamic thresholding (have a higher confidence first and then change confidence gradually)
    \item Normalize the scores only over implicit labels for thresholding and not the entire label space
    \item How about using logit adjustment (post-processing) to address the long-tail in prediction. 
    \item Look at the cost of improving labels in the test set and how we could evaluate this (metric) to take the multiple labels into account. 
    \item Paper title (Hakan's suggestion :D): NOT ALL RELATIONS ARE EQUAL
\end{itemize}

\noindent
\textbf{Oct 5, 2021 - Meeting with Frank}

\begin{itemize}
    \item Look at the test set to see if the model predicts certain implicit relations which are missing in the test ground truth
    \item What can we do to take care of missing labels in evaluation? Maybe annotate them using our matrix annotations ?
    \item Doing this test set cleaning could be a good contribution (no one currently is looking at it or published yet)? Can we make this an extension of this work? 
\end{itemize}

\noindent
\textbf{Sept 30, 2021}

\begin{itemize}
   \item Train with only implicit pseudo labels in the second stage (no ground truth explicit labels)

    \item Train with only explicit ground truth labels with mixup in the second stage
    \item Try thresholding on pseudo-labels. 
    \item Train the model with loss modeling 
    \item Maybe train with mixup in the first stage? 
    \item See what in mixup works best
    \item add state of the art table in the paper
    \item re-write the method section and motivation 
\end{itemize}

\noindent
\textbf{Sept 23, 2021}

\begin{itemize}
    \item Check the statistics of the dataset, how many explicit and implicit labels we have.
    \item Check the performance/confidence of the pseudo-labels.
    \item Check the data augmentation Manifold Mixup performance in both the input and target space. 
    \item Write and collect all results so that it makes sense.  
\end{itemize}

\noindent
\textbf{Sept 16, 2021}

\begin{itemize}
    \item Try Symmetric KL divergence and CE loss in line 20.
    \item Try soft pseudo labels in line 15 for training directly with Symmetric KL/CE/Consistency Loss in line 20.
    \item Use ranking loss (LSEP) for training in line 20 with the matrix annotations and pseudo labels.
    \item See what is similar is semi supervised multi label problems.
    \item Compare it to other multi-label problems / incomplete label problems.
    \item Maybe see if we can define a toy problem for this kind of setting. 
\end{itemize}

\section*{Hakan's questions}
\begin{itemize}
    \item How does our method compare to the prior work in Multi-Label Learning with Incomplete Labels? Eg \cite{bucak2011multi,li2017improving}
        
    \begin{itemize}
        \item \arushi{Basically, in our problem setting there are two multi-label settings - one at the image level and one at the triplet level. At the image level, the multi-labels are the triplets (subject-relation-object) for each image as there can be multiple relevant triplets that can be grounded in the image (\eg man - riding -bike, man - carrying - backpack, bike - next to - bus etc.). At the triplet/pair level, although originally it is treated as a single label problem, we argue that it can have multiple plausible labels for each pair (\eg man - on/walking on -street). Incompleteness of labels can be studied both at this image level and triplet level, but we are currently focusing on the triplet level incompleteness. From my perspective, these papers are more relevant for incompleteness at image level as usually they deal with ranking these labels (\eg )or studying missing labels based on context information etc. (\eg if toothpaste is not annotated and brush is annotated then highly likely that toothpaste is a positive label.) At the triplet level, it is very vague to define the ranking (I am not sure if it makes sense even, I think it's more like a hierarchy). Maybe the context information makes sense and that's what we are trying to do by incorporating label correlations at the pair/triplet level. Due to this vagueness in ranking at triplet level, directly comparing these multi-label learning methods is very hard and also probably hard to incorporate ranking based losses. But it seems very relevant for the image level multi-label problem.}
    \end{itemize}
    
    \item Can we also use low-rank classifiers for learning label correlation? How does our implied labels relate to label correlation?
    \begin{itemize}
        \item \arushi{}
    \end{itemize}
    \item How about the prior work in semi-supervised learning for missing labels \cite{zhao2015semi}?
    \begin{itemize}
        \item \arushi{Thanks for sharing this paper. This looks super relevant and very related! I think we are kind of doing something very similar where we impute missing labels via this implicit pre-training mechanism and then derive a (latent) true labels based on incomplete ground truth labels and the predicted labels.}
    \end{itemize}
    \item What is unique about our problem? How does it differ from other generic multi-label incomplete label tasks? Does labeling object pair give a different twist to the problem?
    \item Many papers use rank based loss functions for incomplete labels (eg see \cite{bucak2011multi,li2017improving})? Can we also use one or what is the advantage of our loss function over the ranking one?
    \begin{itemize}
        \item \arushi{I think we can also experiment with the ranking based loss functions instead of the KL/CE loss in the pseudo-label step. More specifically, this paper has proposed an LSEP loss \cite{li2017improving} which I think can be used for multi-label classification instead of traditional softmax CE loss and still use softmax for prediction during inference time. } 
    \end{itemize}
    \item Can we further improve our method inspired from recent semi-supervised learning methods? Eg using some form of consistency.

\end{itemize}

\subsection{Basura}

\begin{itemize}
    \item Now we predict pseudo labels for explicit set. What if we predict also the explicit relations for implicit once? 
    
    \item Can we define a consistency loss at line 15? Perhaps if predicted implicit verb is $v_i$ for explicit example $v_j$ and if $v_i \nRightarrow v_j$ then we should penalize the model. We should encourage model to predict one of the implicit verbs that implies $v_j$.
    
    \item Perhaps symmetric KL divergence is more meaningful.
    
    \item We can also use the Cross-entropy in Line 20. $-\sum \hat{\bar{p}}_e \times log (\bar{p}_e)$. The good thing about Cross-entropy is that it can also reduce the model entropy (uncertainty). However, this can also be bad in our case. I have a feeling if KL works better than CE loss. Because CE = KL + ENTROPY. Increasing the model entropy can also be good sometimes.

\end{itemize}

\subsection{Dataset Details}
\label{sec.dataset}

For the Visual Genome dataset \cite{krishna2017visual}, \cite{xu2017scene} released a version of the dataset with 50 relations and 150 object categories. These 50 relations are: \emph{above, across, against, along, and, at,  attached to,  behind,  belonging to,  between,  carrying,  covered in, covering, eating,  flying in,  for,  from,  growing on,  hanging from,  has,  holding,  in,  in front of, laying on, looking at,  lying on,  made of,  mounted on,  near,  of,  on,  on back of,  over,  painted on,  parked on, part of,  playing,  riding,  says,  sitting on,  standing on,  to,  under,  using,  walking in,  walking on,  watching,  wearing,  wears,  with.}

Out of these 50 relations, following \cite{collell2018acquiring} we define a set of explicit/spatial and implicit/verb relations. We define explicit relations when the spatial arrangement of objects are implied by the label itself \eg,  ``on",  ``below", ``next to'' and so on.   For implicit relations,  the spatial arrangement of objects is only indirectly implied, ``riding'', ``walking'', ``holding" etc. 

More specifically, for the Visual Genome dataset, the explicit/spatial relations are above, across, against, along, at, behind, between, in, in front of, near, on, over, under and the rest are implicit/verb relations. \arushi{Probably these are loosely defined right now and there could be some others from the list that can be defined as explicit for instance. Maybe it makes more sense if we call the explicit relations as \emph{spatial} relations?}

\arushi{MORE COMMENTS - I will pull the data for the number of samples/pairs for each label/relation. But on second thought I think maybe the dataset in current form does not suffer from long-tail problem (majority and minority) because previous works removed relations with very few samples and hence we are left with 50 relations at the end. So probably I take back the reasoning when I said that the method does better on explicit relations because there are more samples, there must be an imbalance but not that severe I suppose.}

\noindent
\textbf{Dataset Statistics}
\begin{table*}[!ht]

		\resizebox{\textwidth}{!}{
			\begin{tabular}{|c|c |c | c| c| c| c| c| c| c| c|c|c|c|}
				\hline
				
				 Explicit Labels & above&	across&	against&	along& 	at& 	behind&	between&	in&	in front of	&near&	on&	over&	under \\
				\hline 
			
				  \# of Instances & 47341 &	1996 &	3092 &	3624 & 	9903 & 	41356 &	3411 &	251756 &13715	& 96589 &	712409 & 9317 &	22596 \\ \hline
				
				\hline

\end{tabular}}
\caption{No. of Instances for explicit labels, Total: 1217105}
\label{table:dataset}
\end{table*}

\begin{table*}[!ht]

		\resizebox{\textwidth}{!}{
			\begin{tabular}{|c|c |c | c| c| c| c| c| c| c| c|c|c|c|c|c |c | c| c| c| c| c| c| c| c|c|c|c|c|c |c | c| c| c| c| c| c| c|}
				\hline
				
				 Implicit Labels & attached to&	and&	belonging to&	carrying&	covered in &	covering&	eating	&flying in&	for& 	from	&growing on&	hanging from	&has&	holding	&laying on&	looking at \\
				\hline
			
				  \# of Instances & 10190 &	3477 &	3288&	5213&	2312 &	3806&	4688	&1973 &	9145& 	2945& 1853& 9894& 277936& 42722& 3739& 3083 \\ \hline
				
				\hline

\end{tabular}}
\caption{No. of Instances for implicit labels, Total:828901}
\label{table:dataset}
\end{table*}

\begin{table*}[!ht]

		\resizebox{\textwidth}{!}{
			\begin{tabular}{|c|c |c | c| c| c| c| c| c| c| c|c|c|c|c|c |c | c| c| c| c| c| c| c| c|c|c|c|c|c |c | c| c| c| c| c| c| c|}
				\hline
				
				 Implicit Labels & lying on&	made of& 	mounted on	&of	&on back of&	painted on&	parked on&	part of&	playing	&riding	&says&	sitting on& 	standing on&	to	&using	&walking in&	walking on&	watching&	wearing&	wears	&with \\
				\hline
			
				  \# of Instances & 1869& 2380& 2253&  146339. & 1914& 3095& 2721& 2065& 3810& 8856& 2241& 18643& 14185& 2517& 1925& 1740& 4613& 3490& 136099& 15457& 66425 \\ \hline
				
				\hline

\end{tabular}}
\caption{No. of Instances for implicit labels, Total: 828901}
\label{table:dataset}
\end{table*}

\noindent
\textbf{Preliminaries. }Just for the sake of clarity, here we discuss the definition of mutually exclusive and implied-by relation annotations that we annotated in the previous version of the paper. 

Inspired from \cite{ramanathan2015learning}, given a set of unique relation labels, $\mathcal{P}$,  we define two relations between relations.

\noindent
1. \textbf{mutually exclusive relations:} Two relations $i$ and $j$ are considered mutually exclusive if they cannot co-exist for the same object pair. Triplets \emph{(person \textbf{sitting on} grass)} and \emph{(person \textbf{walking on} grass)} will not hold true at the same time. Hence, \textbf{sitting on} and \textbf{walking on} are mutually exclusive relations.
We denote this relation with a matrix $\mathcal{M}$ where $\mathcal{M}_{ij}=1$ when $i$ and $j$ are mutually exclusive, otherwise 0.
 
\noindent
2. \textbf{implied relations:} In an implied relation, relations $i$ implies relation $j$. For instance, \emph{(person \textbf{skate on} skateboard)} implies \emph{(person \textbf{on} skateboard)}, denoting that \textbf{on} is \emph{implied} by \textbf{skate on}, but not vice-versa. 
We denote this relation with a matrix $\mathcal{I}$ where $\mathcal{I}_{ij}=1$ when $i$ implies $j$, otherwise 0.

\noindent
\textbf{Algorithm. } \Cref{algo:vrd} illustrates our method in detail. For each minibatch, we divide the dataset into two subsets $\mathcal{A}$ and $\mathcal{Z}$ with the implicit/verb and explicit/spatial relations respectively. We first train the model on all the triplets/samples in the subset $\mathcal{A}$ using a standard cross-entropy loss or our proposed partial mutually exclusive softmax cross entropy loss. \arushi{Line 8 in \cref{algo:vrd}, I do not as such see the benefit or motivation of using Partially mutual exclusive softmax (PMES) instead of traditional softmax. Maybe PMES will be helpful while pseudo-labeling by predicting the implicit/verb class with a higher probability ? I still have to test this part of the code.} 
After this initial stage of training, we predict pseudo implicit labels for all the samples/pairs in the subset $\mathcal{Z}$. We refine the ground-truth explicit/spatial relation for these pairs with the pseudo implicit labels and define a multi-label relation vector for further training. \textit{Please note that during pseudo label prediction, we force the model to only predict the implicit relations}. At each iteration step, we train the model with the joint losses, $\mathcal{L}_v$ on the implicit set and $\mathcal{L}_e$ on the explicit set and also update the pseudo implicit labels at each step. For $\mathcal{L}_e$, we use the KL divergence loss by treating the multi-label one hot vector as probability targets.

\subsection{Approach}

Let $\mathcal{D}$ denote the entire dataset of training triplets/pairs with $(x,y)$ as the corresponding sample and label pairs where, $x \in R^d$ and $y \in R^n$ with $d$ denoting the feature dimensions and $n$ the total number of relation classes. For the relation label space, we define \textit{implicit/verb}, $\mathcal{V}$ and \textit{explicit/spatial}, $\mathcal{E}$ sets. If the label $y_i$ for an $i^{th}$ instance belongs to the set $\mathcal{V}$ then it is called an implicit/verb label else it is an explicit/spatial label. 

The dataset $\mathcal{D}$ is divided into two subsets based on the ground-truth label $y$ for all the training samples in $\mathcal{D}$. These subsets are defined as:

\[
    \mathcal{D}=  
\begin{cases}
     \mathcal{D_V}  ,& \text{if } y_i \in \mathcal{V} ~\forall i \in N  \\
     \mathcal{D_E} ,& \text{if } y_i \in \mathcal{E} ~\forall i \in N  
 
    \label{eq.datasubset}
\end{cases}
\]

where $N$ are the total number of training samples in $\mathcal{D}$ with $N_V$ samples in the subset $\mathcal{D_V}$ and $N_E$ samples in the subset $\mathcal{D_E}$. 

\noindent 
\textbf{Warmup Training. }
We perform warmup training using cross-entropy Loss on implicit label set, $\mathcal{D_V}$ as:
\begin{equation}
    \mathcal{L_{V}} = \sum_{i=1}^{N_V} \mathcal{L}_{CE}(p_{model}(\bm{x}_i; \theta), y_i)
\end{equation}

After the warmup training, pseudo-labels are predicted for the samples in subset $\mathcal{D_E}$. These pseudo-labels can be incorporated into the training via different label refinement techniques and loss functions. 

\noindent
\textbf{\textit{Pseudo Label refinement using ground truth.}
}
For a sample $x_i$ in the subset $\mathcal{D_E}$, we predict the hard pseudo-label as : 

\begin{equation}
    \hat{y}_i = \argmax(p_{model}(\bm{x}_i; \theta))
\end{equation}
We then refine the hard pseudo-label with the ground-truth label $y_i$ for $x_i$ in $\mathcal{D_E}$. The final multi-label valued one-hot vector, $\bar{y}_i$, is then given as :

\begin{equation}
    \bar{y}_i = \beta * \hat{y}_i + (1 - \beta) * y_i
\end{equation}

where $\hat{y}_i$ and $y_i$ are the one-hot label vectors and $\beta$ is the weight for each one-hot vector. 

The loss function for training on $\mathcal{D_E}$ with $\bar{y}_i$ is given by - 

% \begin{equation}
%     \mathcal{L_{E}} = \sum_{i=1}^{N_E} \mathcal{L}_{CE}(p_{model}(\bm{x}_i; \theta), \bar{y}_i)
% \end{equation}
 
%  or 
 
\begin{equation}
    \mathcal{L_{E}} = \sum_{i=1}^{N_E} \mathcal{L}_{KL}(p_{model}(\bm{x}_i; \theta), \bar{y}_i)
    \label{eq.exploss}
\end{equation}

where, $\mathcal{L}_{KL}$ is the KL-divergence loss between the predicted probabilities and the ground-truth probabilities. The choice of the loss function in \Cref{eq.exploss} is yet to be explored for a more comprehensive and principled training procedure. These include jensen-shannon divergence, consistency loss, multi-label cross entropy loss and log-sum exponential pairwise ranking loss. \Cref{algo:vrd} summarizes our full method in detail. 

\noindent
\textbf{\textit{Consistency training with Soft Pseudo-Labels}}

\noindent
\textit{\textbf{Data Augmentations}
}
Manifold Mixup

\noindent
\textbf{Loss Modeling for pseudo-label selection. }

After the initial warmup training of the model with only the implicit subset of labels, we calculate the loss values of the entire training set with respect to the ground truth / true label. More specifically, we have a loss value $l_i$ for each sample $i$ in the training set. 

\begin{equation}
    l_i =  \mathcal{L}_{CE}(p_{model}(\bm{x}_i; \theta), y_i)
\end{equation}

We normalize the loss values $l_i$ to be between 0 and 1. Standard training with the implicit labels perform poorly or have high loss values for the pairs of explicit labels which are hard to classify with only implicit label training. If the model is not confident about it's prediction in the explicit set for a pair, then it is considered as a hard sample to be learned with a higher loss value.

\begin{table*}[!ht]

		\resizebox{\textwidth}{!}{
			\begin{tabular}{|c|c |c | c| c| c| c| c| c| c| c|}
				\hline
				& & \multicolumn{3}{c|}{relation Classification} &\multicolumn{3}{c|}{Scene Graph Classification} & \multicolumn{3}{c|}{Scene Graph Detection }\\
				
				 Models & Method & mR@20 & mR@50 & mR@100 & mR@20 & mR@50 & mR@100  & mR@20 & mR@50 & mR@100  \\
				\hline\hline 
				% VLK \cite{lu2016visual} & 8.45 & - & 3.36  & 3.75 & - & - & 3.13 & 3.52 & - & -   \\
				% VTransE \cite{zhang2017visual} & - & -  & 2.65  & 3.51 & - & - &  1.71 & 2.14 & - & -   \\
				Motif-TDE & CE-Loss & 17.85 & 24.75 & 28.70 & 9.80 & 13.21 & 15.06 & 6.58 & 8.94 & 10.99 \\ \hline
				Motif-TDE & \cref{algo:vrd}, implicit train only & 18.24 & 24.93 & 28.71 & 9.79 & 12.99 & 14.66 & 6.49  & 8.97 & 10.88 \\ 
				% Motif-TDE & \cref{algo:vrd} & 21.44 & 28.15 & 31.16 & & & &  && \\ \hline 
				Motif-TDE & \cref{algo:vrd}, w/o MixUp & 18.26 & 24.23 & 27.48 &  &  &  &  && \\ 
				
				Motif-TDE & \cref{algo:vrd}  w/ Soft Pseudo Labels-KL \& Manifold MixUp (input and target) & 20.76 & 27.18 & 30.33 &  & &  &  & & \\ 
				
				Motif-TDE & \cref{algo:vrd} w/ Soft Pseudo Labels-MSE \& Manifold MixUp (input and target) & 17.97 & 24.54 & 28.19 &  &  & &  & & \\
				
				Motif-TDE & \cref{algo:vrd} w/ Manifold MixUp (input and target) & 20.71 & 27.53 & 30.68 & 11.16 & 14.59 & 16.21 & 8.12 &10.75 & 12.90\\
				Motif-TDE &\cref{algo:vrd} w/ Manifold MixUp (input and target)-LossThreshold($<$0.5) & 19.02 & 25.92 & 29.40 &   & &   &   &  &  \\

				Motif-TDE &\cref{algo:vrd} w/ Manifold MixUp-AllSamples (input and target)-ConfThreshold(0.5) & 18.90 & 25.32 & 28.58 &   & &   &   &  &  \\ 
				Motif-TDE &\cref{algo:vrd} w/ Manifold MixUp - AllSamples (input and target)-LossThreshold($<$0.5) & 19.90 & 26.35 & 29.26 &   & &   &   &  &  \\ 
				Motif-TDE &\cref{algo:vrd} w/ Manifold MixUp - AllSamples (input and target)-LossThreshold($<$0.7 + $>$0.7) & 21.21 & 27.04 & 29.66 &   & &   &   &  &  \\\hline
				Motif-TDE & \cref{algo:vrd} w/ Manifold MixUp-AllSamples (input and target) & 21.26 & 27.14 & 29.68 &  & &  &  & & \\ 
				
				Motif-TDE &\cref{algo:vrd} w/ Manifold MixUp - AllSamples (input and target) + ConfThreshold(0.5) & 20.91 & 26.76 & 29.61 &   & &   &   &  &  \\
				
				Motif-TDE &\cref{algo:vrd} w/ LogitAdjPseudo+Manifold MixUp - AllSamples (input and target) & 20.99 & 26.74 & 29.29 &   & &   &   &  &  \\

				Motif-TDE &\cref{algo:vrd} w/ LogitAdjPseudo+Manifold MixUp - AllSamples (input and target) + ConfThreshold(0.5) & 21.00 & 26.95 & 29.57 &   & &   &   &  &  \\
				
				Motif-TDE &\cref{algo:vrd} w/ LogitAdjPseudo+Manifold MixUp - AllSamples (input and target) + ConfThreshold(0.7) & 21.15 & 26.91 & 29.57 &   & &   &   &  &  \\

				\hline

				Motif-TDE & \cref{algo:vrd} w/ BCE Loss, implicit train only & 20.63 & 26.15 & 29.10 & & & &  && \\ \hline \hline
				
				Motif & CE-Loss & 11.46 & 14.60 & 15.84 & 6.50 & 8.02 & 8.51 & 4.36 & 5.83 & 7.08 \\ \hline
				Motif &\cref{algo:vrd}, implicit train only & 11.52 & 14.56 & 15.77 & 7.08 & 8.81 & 9.47 &4.21 & 5.61 & 6.92 \\
				Motif & \cref{algo:vrd}  w/ Soft Pseudo Labels \& Manifold MixUp (input and target) & 10.33 & 12.55 & 13.28 &  & &  &  & & \\ 
				Motif &\cref{algo:vrd} w/ Manifold MixUp (input and target) & 12.62 & 15.73 & 16.93 & 7.01  & 8.54 &  9.09 & 4.64  & 6.31 & 7.84 \\ 
				Motif &\cref{algo:vrd} w/ Manifold MixUp-AllSamples (input and target)-ConfThreshold(0.5) & 11.54 & 14.45 & 15.66 &   & &   &   &  &  \\ 
				Motif &\cref{algo:vrd} w/ Manifold MixUp (input and target)-LossThreshold(0.5) & 12.30 & 15.38 & 16.71 &   & &   &   &  &  \\ 
				
				Motif &\cref{algo:vrd} w/ Manifold MixUp - AllSamples (input and target)-LossThreshold($<$0.7 + $>$0.7) & 11.58 & 14.49 & 15.56 &   & &   &   &  &  \\ \hline
				
				Motif & \cref{algo:vrd} w/ Manifold MixUp-AllSamples (input and target) & 11.60 & 14.43 & 15.47 &  & &  &  & & \\  
				
				Motif &\cref{algo:vrd} w/ LogitAdjPseudo+Manifold MixUp - AllSamples (input and target) & 11.67 & 14.54 & 15.72 &   & &   &   &  &  \\
			
				Motif &\cref{algo:vrd} w/ LogitAdjPseudo+Manifold MixUp - AllSamples (input and target) + ConfThreshold(0.5) & 11.76 & 14.61 & 15.70 &   & &   &   &  &  \\

				\hline
				Motif & \cref{algo:vrd} w/ BCE Loss, implicit train only & 11.86  & 15.28 & 16.84 & & & &  && \\ \hline
				
				\hline

\end{tabular}}
\caption{Performance on the all test split of the Visual Genome dataset.}
\label{table:zeroshotvrd}
\end{table*}

\begin{table*}[!ht]

		\resizebox{\textwidth}{!}{
			\begin{tabular}{|c|c |c | c| c| c| c| c| c| c| c|}
				\hline
				& & \multicolumn{3}{c|}{relation Classification} &\multicolumn{3}{c|}{Scene Graph Classification} & \multicolumn{3}{c|}{Scene Graph Detection }\\
				
				 Models & Method & Head(16) & Middle(17) & Tail(17) & Head(16) & Middle(17) & Tail(17)   & Head(16) & Middle(17) & Tail(17)  \\
				\hline\hline 
				% VLK \cite{lu2016visual} & 8.45 & - & 3.36  & 3.75 & - & - & 3.13 & 3.52 & - & -   \\
				% VTransE \cite{zhang2017visual} & - & -  & 2.65  & 3.51 & - & - &  1.71 & 2.14 & - & -   \\

				Motif-TDE & \cref{algo:vrd} w/ Manifold MixUp - AllSamples (input and target) &  40.63 & 36.61 & 12.54 & & &  & & & \\

	            Motif-TDE & \cref{algo:vrd} w/ Manifold MixUp - AllSamples (input and target)+ ConfThreshold(0.5)  &  41.15 & 36.13 & 12.65 & & &  & & & \\

				Motif-TDE &\cref{algo:vrd} w/ LogitAdjPseudo+Manifold MixUp - AllSamples (input and target) + ConfThreshold(0.7) & 41.42 & 34.23 & 13.72 &   & &   &   &  &  \\

				\hline

\end{tabular}}
\caption{mR@100 Performance on the separate class sets of the Visual Genome dataset. }
\label{table:zeroshotvrd}
\end{table*}

\begin{table*}[!ht]

		\resizebox{\textwidth}{!}{
			\begin{tabular}{|c|c |c | c| c| c| c| c| c| c| c|}
				\hline
				& & \multicolumn{3}{c|}{relation Classification} &\multicolumn{3}{c|}{Scene Graph Classification} & \multicolumn{3}{c|}{Scene Graph Detection }\\
				
				 Models & Method & R@20 & R@50 & R@100 & R@20 & R@50 & R@100 & R@20 & R@50 & R@100  \\
				\hline\hline 
				% VLK \cite{lu2016visual} & 8.45 & - & 3.36  & 3.75 & - & - & 3.13 & 3.52 & - & -   \\
				% VTransE \cite{zhang2017visual} & - & -  & 2.65  & 3.51 & - & - &  1.71 & 2.14 & - & -   \\
				Motif-TDE & CE-Loss & 33.38 & 45.88 & 51.25 & 20.47 & 26.31 & 28.79 & 11.92 & 16.56 & 20.15 \\ \hline
				Motif-TDE & \cref{algo:vrd}, implicit train only & 34.93 & 46.53 & 51.54 & 23.09 & 29.37 & 31.72 & 13.22  &18.31 & 22.00 \\
				% Motif-TDE & \cref{algo:vrd} & 28.14 & 36.56 & 40.13 & & & &  && \\ \hline 
				Motif-TDE & \cref{algo:vrd}, w/o MixUp & 28.10 & 39.10 & 44.31 &  &  &  &  && \\ 
				
				Motif-TDE & \cref{algo:vrd}  w/ Soft Pseudo Labels-KL \& Manifold MixUp (input and target) & 24.62 & 30.93 & 33.76 &  & &  &  & & \\ 
				Motif-TDE & \cref{algo:vrd} w/ Soft Pseudo Labels-MSE \& Manifold MixUp (input and target) & 33.59 & 45.75 & 51.03 &  &  & &  & & \\
				Motif-TDE & \cref{algo:vrd} w/ Manifold MixUp (input and target) & 28.37 & 38.15 & 42.56 & 20.08 &25.48  &27.48 & 9.51  & 13.17 & 15.79\\ 
				Motif-TDE &\cref{algo:vrd} w/ Manifold MixUp (input and target)-LossThreshold($<$0.5) & 29.57 & 39.78 & 44.50 &   & &   &   &  &  \\\hline
				
				Motif-TDE &\cref{algo:vrd} w/ Manifold MixUp-AllSamples (input and target)-ConfThreshold(0.5) & 36.54 & 48.66 & 53.50 &   & &   &   &  &  \\
				Motif-TDE &\cref{algo:vrd} w/ Manifold MixUp - AllSamples (input and target)-LossThreshold(0.5) & 32.94 & 43.37 & 47.81 &   & &   &   &  &  \\ 
				Motif-TDE &\cref{algo:vrd} w/ Manifold MixUp - AllSamples (input and target)-LossThreshold($<$0.7 + $>$0.7) & 33.92 & 43.76 & 47.68 &   & &   &   &  &  \\ \hline
				
				Motif-TDE & \cref{algo:vrd} w/ Manifold MixUp - AllSamples (input and target) & 33.36 & 43.53 & 47.44 & &  & &  &  & \\
				
				Motif-TDE &\cref{algo:vrd} w/ Manifold MixUp - AllSamples (input and target) + ConfThreshold(0.5) & 33.37 & 43.65 & 47.77 &   & &   &   &  &  \\

				Motif-TDE &\cref{algo:vrd} w/ LogitAdjPseudo+Manifold MixUp - AllSamples (input and target) & 35.04 & 44.12 & 47.38 &   & &   &   &  &  \\
				
				Motif-TDE &\cref{algo:vrd} w/ LogitAdjPseudo+Manifold MixUp - AllSamples (input and target) + ConfThreshold(0.5) & 34.97 & 44.16 & 47.55 &   & &   &   &  &  \\
				
				Motif-TDE &\cref{algo:vrd} w/ LogitAdjPseudo+Manifold MixUp - AllSamples (input and target) + ConfThreshold(0.7) & 35.16 & 44.55 & 48.15 &   & &   &   &  &  \\

				\hline
			
				Motif-TDE & \cref{algo:vrd} w/ BCE Loss, implicit train only & 27.17 & 37.75 & 43.86 & & & &  && \\ \hline \hline

				Motif & CE-Loss & 59.64 & 66.11 & 67.96 & 36.02 & 39.25 & 40.07 & 25.42 & 32.45 & 37.26 \\ \hline
				Motif &\cref{algo:vrd}, implicit train only & 57.42 & 64.37 & 66.43 & 35.42 & 38.79 & 39.66 &23.70 &30.74  &  35.62\\
				Motif & \cref{algo:vrd}  w/ Soft Pseudo Labels \& Manifold MixUp (input and target) & 58.66 & 64.69 & 66.22 &  & &  &  & & \\ 
				Motif & \cref{algo:vrd} w/ Manifold MixUp (input and target) & 58.77 & 65.29 & 67.05 & 35.49 & 38.71 & 39.51 & 24.63  & 31.52 & 36.42 \\ 
				Motif &\cref{algo:vrd} w/ Manifold MixUp (input and target)-LossThreshold(0.5) & 58.47 & 65.07 & 66.94 &   & &   &   &  &  \\
				Motif &\cref{algo:vrd} w/ Manifold MixUp-AllSamples (input and target)-ConfThreshold(0.5) & 59.03 & 65.58 & 67.45 &   & &   &   &  &  \\ 
			
				Motif &\cref{algo:vrd} w/ Manifold MixUp - AllSamples (input and target)-LossThreshold($<$0.7 + $>$0.7) & 59.17 & 65.63 & 67.41 &   & &   &   &  &  \\ \hline
				
				Motif & \cref{algo:vrd} w/ Manifold MixUp-AllSamples (input and target) & 59.05 & 65.48 & 67.22 &  & &  &  & & \\ 
					
				Motif &\cref{algo:vrd} w/ LogitAdjPseudo+Manifold MixUp - AllSamples (input and target) & 59.09 & 65.60 & 67.40 &   & &   &   &  &  \\
			
				Motif &\cref{algo:vrd} w/ LogitAdjPseudo+Manifold MixUp - AllSamples (input and target) + ConfThreshold(0.5) & 59.17 & 65.64 & 67.43 &   & &   &   &  &  \\
				\hline
		
			    Motif & \cref{algo:vrd} w/ BCE Loss, implicit train only & 56.25 & 64.28 & 66.85 & & & &  && \\ \hline \hline
				
				\hline

\end{tabular}}
\caption{Performance on the all test split of the Visual Genome dataset.}
\label{table:zeroshotvrd}
\end{table*}

\begin{table*}[!ht]

		\resizebox{\textwidth}{!}{
			\begin{tabular}{|c|c |c | c| c| c| c| c| c| c| c|}
				\hline
				& & \multicolumn{3}{c|}{relation Classification} &\multicolumn{3}{c|}{Scene Graph Classification} & \multicolumn{3}{c|}{Scene Graph Detection }\\
				
				 Models & Method & zsR@20 & zsR@50 & zsR@100 & zsR@20 & zsR@50 & zsR@100  & zsR@20 & zsR@50 & zsR@100  \\
				\hline\hline 
				% VLK \cite{lu2016visual} & 8.45 & - & 3.36  & 3.75 & - & - & 3.13 & 3.52 & - & -   \\
				% VTransE \cite{zhang2017visual} & - & -  & 2.65  & 3.51 & - & - &  1.71 & 2.14 & - & -   \\
				Motif-TDE & CE-Loss & 8.28&	14.31	&18.04& 1.91	&2.95&	4.10& 1.54	&2.33	&3.03 \\ \hline
				Motif-TDE & \cref{algo:vrd}, implicit train only & 7.83 & 12.71 & 16.30 & 1.71 &2.63  & 3.37 & 1.10  &1.83 & 2.58\\
				Motif-TDE & \cref{algo:vrd}, w/o MixUp & 7.35 & 11.68 & 14.81 &  &  &  &  && \\

				Motif-TDE & \cref{algo:vrd}  w/ Soft Pseudo Labels-KL \& Manifold MixUp (input and target) & 8.25 & 12.78 & 15.60 &  & &  &  & & \\ 
				
				Motif-TDE & \cref{algo:vrd} w/ Soft Pseudo Labels-MSE \& Manifold MixUp (input and target) & 7.72 & 12.48 & 15.60 &  &  & &  & & \\ 
				
				Motif-TDE & \cref{algo:vrd} w/ Manifold MixUp (input and target) &  8.28 & 13.30 & 16.10 & 1.90 & 2.99 & 3.73 & 1.65 &2.55& 3.13\\
				Motif-TDE &\cref{algo:vrd} w/ Manifold MixUp (input and target)-LossThreshold($<$0.5) & 8.33 & 12.92 & 16.05 &   & &   &   &  &  \\
				
				Motif-TDE &\cref{algo:vrd} w/ Manifold MixUp-AllSamples (input and target)-ConfThreshold(0.5) & 9.48 & 14.86 & 17.72 &   & &   &   &  &  \\
				Motif-TDE &\cref{algo:vrd} w/ Manifold MixUp - AllSamples (input and target)-LossThreshold(0.5) & 9.23 & 14.14 & 17.24 &   & &   &   &  &  \\ 
				Motif-TDE &\cref{algo:vrd} w/ Manifold MixUp - AllSamples (input and target)-LossThreshold($<$0.7 + $>$0.7) & 9.06 & 14.02 & 17.17 &   & &   &   &  &  \\\hline
				
				Motif-TDE & \cref{algo:vrd} w/ Manifold MixUp - AllSamples (input and target) &  9.33 & 14.43 & 17.21 & & &  & & & \\

	            Motif-TDE & \cref{algo:vrd} w/ Manifold MixUp - AllSamples (input and target) &  9.21 & 14.29 & 16.91 & & &  & & & \\

				Motif-TDE &\cref{algo:vrd} w/ LogitAdjPseudo+Manifold MixUp - AllSamples (input and target) & 8.82 & 13.76 & 16.60 &   & &   &   &  &  \\
				
				Motif-TDE &\cref{algo:vrd} w/ LogitAdjPseudo+Manifold MixUp - AllSamples (input and target) + ConfThreshold(0.5) & 8.99 & 13.97 & 16.66 &   & &   &   &  &  \\
				
				Motif-TDE &\cref{algo:vrd} w/ LogitAdjPseudo+Manifold MixUp - AllSamples (input and target) + ConfThreshold(0.7) & 9.21 & 14.32 & 17.17 &   & &   &   &  &  \\

				\hline 
				Motif-TDE & \cref{algo:vrd} w/ BCE Loss, implicit train only & 7.95 & 11.76 & 14.19 & & & &  && \\ \hline \hline
				Motif & CE-Loss & 5.79  &	11.02	& 14.74 & 1.06	& 2.18 &	3.07 & 0.02	& 0.08	& 0.24 \\ \hline
				Motif &\cref{algo:vrd}, implicit train only & 4.18 & 8.79 & 11.55 & 0.85 & 1.70 & 2.37 &0.02 &0.02  & 0.16 \\
				Motif & \cref{algo:vrd}  w/ Soft Pseudo Labels \& Manifold MixUp (input and target) & 4.77 & 9.13 & 11.82 &  & &  &  & & \\ 
				Motif & \cref{algo:vrd} w/ Manifold MixUp (input and target)  & 4.93  & 9.41 & 12.25 & 0.95 & 1.70 & 2.37 & 0.02  & 0.06 & 0.22\\

				Motif &\cref{algo:vrd} w/ Manifold MixUp (input and target)-LossThreshold(0.5) & 5.13 & 9.85 & 12.94 &   & &   &   &  &  \\ 
				
				Motif &\cref{algo:vrd} w/ Manifold MixUp-AllSamples (input and target)-ConfThreshold(0.5) & 5.18 & 9.96 & 13.24 &   & &   &   &  &  \\ 
				Motif &\cref{algo:vrd} w/ Manifold MixUp - AllSamples (input and target)-LossThreshold($<$0.7 + $>$0.7) & 4.93 & 9.38 & 12.35 &   & &   &   &  &  \\ \hline

				Motif & \cref{algo:vrd} w/ Manifold MixUp-AllSamples (input and target) & 4.93 & 9.06 & 12.05 &  & &  &  & & \\ 
				
				Motif &\cref{algo:vrd} w/ LogitAdjPseudo+Manifold MixUp - AllSamples (input and target) & 4.99 & 9.48 & 12.59 &   & &   &   &  &  \\
			
				Motif &\cref{algo:vrd} w/ LogitAdjPseudo+Manifold MixUp - AllSamples (input and target) + ConfThreshold(0.5) &5.06 & 9.53 & 12.77&   & &   &   &  &  \\

				\hline
				Motif & \cref{algo:vrd} w/ BCE Loss, implicit train only & 3.16 & 7.51 & 11.49 & & & &  && \\ \hline

				\hline

\end{tabular}}
\caption{Performance on the zero-shot split of the Visual Genome dataset. }
\label{table:zeroshotvrd}
\end{table*}

\section{Supplementary Results}

\begin{table*}[!ht]

		\resizebox{\textwidth}{!}{
			\begin{tabular}{c|c |c | c| c| c| c| c| c| c| c}
				\hline
				& & \multicolumn{3}{c|}{relation Classification} &\multicolumn{3}{c|}{Scene Graph Classification} & \multicolumn{3}{c}{Scene Graph Detection }\\
				
				 Models & Method & mR@20 & mR@50 & mR@100 & mR@20 & mR@50 & mR@100  & mR@20 & mR@50 & mR@100  \\
				\hline
				% VLK \cite{lu2016visual} & 8.45 & - & 3.36  & 3.75 & - & - & 3.13 & 3.52 & - & -   \\
				% VTransE \cite{zhang2017visual} & - & -  & 2.65  & 3.51 & - & - &  1.71 & 2.14 & - & -   \\
				
				\multirow{3}{*}{IMP \cite{xu2017scene}} & Baseline &  8.85 & 10.97 & 11.77 & 5.4 & 6.4& 6.74 &2.2 &3.29& 4.14 \\ 
				 & LIL  & 11.60 & 14.19  & 15.36 & 6.33 & 7.60 & 8.13 & 6.48  & 7.70 & 8.16 \\ 
				& LIP & 12.25 & 14.59 & 15.33 & 7.11 & 7.97 & 8.29 & 6.94 & 7.81 & 8.12  \\\hline

				% Motif & CE-Loss & 11.46 & 14.60 & 15.84 & 6.50 & 8.02 & 8.51 & 4.36 & 5.83 & 7.08  \\ 
				% Motif & Ours & &  &  &  &  &  &  &  &  \\ \hline
				
    			\multirow{3}{*}{Motif-TDE-Sum \cite{tang2020unbiased}} & Baseline & 17.85 & 24.75 & 28.70 & 9.80 & 13.21 & 15.06 & 6.58 & 8.94 & 10.99 \\ 
				 & LIL  & 18.24 & 24.93 & 28.71 & 9.79 & 12.99 & 14.66 & 6.49  & 8.97 & 10.88 \\ 
				 & LIP  & \textbf{21.26} & \textbf{27.14} & \textbf{29.68} & \textbf{11.25} & \textbf{14.25} & \textbf{15.68}  &\textbf{8.37} & \textbf{10.42} & \textbf{11.81} \\ \hline

				\multirow{3}{*}{VCTree \cite{tang2018learning}} & Baseline & 13.07 & 16.53 & 17.77 & 8.5&  10.53 & 11.24& 5.31& 7.16 & 8.35 \\ 
				%  & LIL & 12.70 & 16.21 & 17.62 &  &  &  &  &  &  \\ 
				 & LIL & 17.98 & 21.74 & 23.14 & R(test) & R & R & R(daisy2-det) & R & R \\ 
			
				 & LIP & R(vr) & R & R & R(pr) & R &  R &  &  &  \\ \hline

				\multirow{3}{*}{VCTree-EBM \cite{suhail2021energy}} & Baseline &14.2&  18.19& 19.72& 10.4 &12.54& 13.45& 5.67 &7.71 &9.1   \\ 
				 & LIL & 18.69 & 22.76 & 24.40 & 12.88  & 14.59 & 15.63 & 7.14  & 9.44 & 10.92 \\ 
			
				 & LIP & 21.02 & 24.86 & 26.46 & 13.96 & 16.21 & 17.12 & 7.77 & 10.10 & 11.76 \\ \hline
				
				\multirow{3}{*}{VCTree-TDE \cite{tang2020unbiased}} & Baseline & 16.3 & 22.85 & 26.26 & 11.85 & 15.81 & 17.99 & 6.59& 8.99& 10.78 \\ 
				% VCTree-TDE & EBM-Loss & 19.87 & 26.66 & 29.97 & 13.86 & 18.2 & 20.45& 7.1& 9.69& 11.6  \\ 
				& LIL & 19.58 & 26.29 & 29.86  & 14.12  & 19.01 & 21.56 & 7.40  & 9.58 & 10.94
				\\
				
                 & LIP & 22.15 & 28.07 & 30.58  & 17.76 & 21.95 & 23.63 & 8.41  & 10.32 & 11.46 \\ \hline

\end{tabular}}
\caption{SOTA on Mean Recall:Visual Genome dataset.}
\label{table:zeroshotvrd}
\end{table*}

\begin{table*}[!ht]

		\resizebox{\textwidth}{!}{
			\begin{tabular}{c|c |c | c| c| c| c| c| c| c| c}
				\hline
				& & \multicolumn{3}{c|}{relation Classification} &\multicolumn{3}{c|}{Scene Graph Classification} & \multicolumn{3}{c}{Scene Graph Detection }\\
				
				 Models & Method & zsR@20 & zsR@50 & zsR@100 & zsR@20 & zsR@50 & zsR@100  & zsR@20 & zsR@50 & zsR@100  \\
				\hline
				% VLK \cite{lu2016visual} & 8.45 & - & 3.36  & 3.75 & - & - & 3.13 & 3.52 & - & -   \\
				% VTransE \cite{zhang2017visual} & - & -  & 2.65  & 3.51 & - & - &  1.71 & 2.14 & - & -   \\

				\multirow{3}{*}{IMP \cite{xu2017scene}} & Baseline &  12.17 & 17.66 & - & 2.09& 3.3 &- & 0.14& 0.39  & - \\ 
				& LIL  & 5.75 & 8.07  & 9.38 & 1.09 & 1.80 & 2.06 & 0.88 & 1.71 & 2.00 \\ 
				 & LIP &7.12  & 10.50 & 12.33 & 1.57 & 2.32 & 2.81 & 1.52 & 2.48 & 2.97 \\\hline
		
				% Motif & CE-Loss & 11.46 & 14.60 & 15.84 & 6.50 & 8.02 & 8.51 & 4.36 & 5.83 & 7.08  \\ 
				% Motif & Ours & &  &  &  &  &  &  &  &  \\ \hline
				
    			\multirow{3}{*}{Motif-TDE-Sum \cite{tang2020unbiased}} & Baseline & 8.28&	14.31	&\textbf{18.04}& \textbf{1.91}	&2.95&	\textbf{4.10}& 1.54	&2.33	&3.03 \\ 
				& LIL  & 7.83 & 12.71 & 16.30 & 1.71 &2.63  & 3.37 & 1.10  &1.83 & 2.58 \\ 
				 & LIP  & \textbf{9.33} & \textbf{14.43} & 17.21 & 1.87 & \textbf{2.99} & 3.76 & \textbf{2.06}& \textbf{3.05} & \textbf{3.72} \\ \hline

				\multirow{3}{*}{VCTree \cite{tang2018learning}} & Baseline &  1.43 & 4 & -& 0.39& 1.2 & - & 0.19& 0.46 & - \\ 
			 %  & LIL & 5.35 & 10.51 & 14.18 &  &  &  &  &  &  \\ 
			   & LIL & 1.51 & 3.66 & 5.09 &  &  &  &  &  &  \\ 
			
				 & LIP &  & &  &  &  &  &  &  &  \\ \hline

				% \multirow{3}{*}{VCTree-EBM \cite{suhail2021energy}} & Baseline & 2.25 & 5.36 & - & 0.87& 1.87 & - & 0.21& 0.54 & -     \\ 
				%  & LIL &  &  &  &  0.70  & 1.51 & 1.86 & 0.07 & 0.24 & 0.50 \\ 
			
				%  & LIP &  &  &  & 0.19 &  0.39 & 0.60 & 0.13 & 0.29 & 0.51 \\ \hline

				\multirow{3}{*}{VCTree-TDE \cite{tang2020unbiased}} & Baseline &  8.98 & 14.52 & - & 3.16 & 4.97 & - & 1.47 & 2.3 & - \\ 
				% VCTree-TDE & EBM-Loss & 19.87 & 26.66 & 29.97 & 13.86 & 18.2 & 20.45& 7.1& 9.69& 11.6  \\ 
				& LIL &  8.56 & 13.54 & 17.36 & 3.66 & 5.55 & 7.10 & 1.85 & 2.74 & 3.66 \\
				
                 & LIP &9.11  & 13.52 &  16.24 & 4.26 & 6.20 & 7.29 & 2.24 & 3.25 & 3.94 \\ \hline

\end{tabular}}
\caption{SOTA on Zero Shot Recall:Visual Genome dataset.}
\label{table:zeroshotvrd}
\end{table*}

\begin{table*}[!ht]

		\resizebox{\textwidth}{!}{
			\begin{tabular}{c|c |c | c| c| c| c| c| c| c| c}
				\hline
				& & \multicolumn{3}{c|}{relation Classification} &\multicolumn{3}{c|}{Scene Graph Classification} & \multicolumn{3}{c}{Scene Graph Detection }\\
				
				 Models & Method & R@20 & R@50 & R@100 & R@20 & R@50 & R@100  & R@20 & R@50 & R@100  \\
				\hline
				% VLK \cite{lu2016visual} & 8.45 & - & 3.36  & 3.75 & - & - & 3.13 & 3.52 & - & -   \\
				% VTransE \cite{zhang2017visual} & - & -  & 2.65  & 3.51 & - & - &  1.71 & 2.14 & - & -   \\
				
				IMP & CE-Loss &  54.34 &61.05& 63.06&  34.02& 37.39& 38.26&  16.34& 23.64 &28.71  \\ 
				IMP & Ours, LIL & 29.98 & 32.69 & 33.48 & 18.96 & 20.36 & 20.69 &16.46 & 17.67 & 18.00 \\ 
				IMP & Ours, LIP & 33.46 & 37.88 & 39.40 & 22.76 & 25.19 & 25.92 &19.25  & 21.18 & 21.81 \\ \hline
							
				Motif & CE-Loss &  59.64 & 66.11 & 67.96 & 36.02 & 39.25 & 40.07 & 25.42 & 32.45 & 37.26\\ 
				Motif & Ours & &  &  &  &  &  &  &  &  \\ \hline
				
    			Motif-TDE & CE-Loss & 33.38 & 45.88 & 51.25 & 20.47 & 26.31 & 28.79 & 11.92 & 16.56 & 20.15  \\ 
				Motif-TDE & Ours & 33.36 & 43.53 & 47.44 & 24.31 & 29.91 & 31.75 & 14.59 & 17.96 & 19.70 \\ \hline
				
                VCTree & CE-Loss & 59.82 & 65.93 & 67.57 & 41.49& 45.16& 46.1& 24.9& 32.02& 36.3 \\ 
				VCTree & Ours, LIN only & 32.82 & 35.17 & 35.73 &  &  &  &  &  &  \\ 
				VCTree & Ours, LIN+Mixup+KL &  & &  &  &  &  &  &  &  \\ 
				VCTree & Ours, LIN+Mixup-Allsamples+KL & &  &  & 23.09 & 24.48 & 24.78 & 14.97 & 16.16 & 16.48 \\ \hline

				VCTree & EBM-Loss & 57.31 & 63.99& 65.84 & 40.31 &44.72 &45.84 & 24.21 &31.36& 35.87    \\ 
				VCTree & Ours, LIN only & 32.55 & 35.06 & 35.67 & 23.59 & 25.01 & 25.33  & 15.54 & 19.33 & 21.43 \\ 
				VCTree & Ours, LIN+Mixup+KL & 36.26 & 41.04 & 42.68 &  &  &  &  &  &  \\
				VCTree & Ours, LIN+Mixup-Allsamples+KL & 38.18 & 44.52 & 46.45 & 29.46 & 32.89 & 33.86 & 17.13 & 22.29 & 25.53 \\ \hline
			
				VCTree-TDE & CE-Loss & 40.12 & 50.83 &54.91 & 26 &33.03 &35.97 & 13.97& 19.43 &23.34  \\ 
				% VCTree-TDE & EBM-Loss & 41.62 & 51.22& 54.29&  29.53 &36.49& 38.92&  14.66 &20.55& 24.74  \\ 
				VCTree-TDE & Ours, LIN only  & 36.90 & 47.62 & 52.03  & 25.67 & 32.83 & 35.76 & 15.20 & 19.00 & 20.98 \\ 
				VCTree-TDE & Ours & 33.80 & 43.04  &  46.71 & 28.51  & 34.06 & 35.75 &  15.69 & 19.05 & 20.71 \\ 
				
				\hline

\end{tabular}}
\caption{SOTA on Regular Recall:Visual Genome dataset.}
\label{table:zeroshotvrd}
\end{table*}

\begin{table*}[!ht]

		\resizebox{\textwidth}{!}{
			\begin{tabular}{c|c |c | c| c| c| c| c| c| c| c}
				\hline
				& & \multicolumn{3}{c|}{relation Classification} &\multicolumn{3}{c|}{Scene Graph Classification} & \multicolumn{3}{c}{Scene Graph Detection }\\
				
				 Models & Method & zsR@20 & zsR@50 & zsR@100 & zsR@20 & zsR@50 & zsR@100  & zsR@20 & zsR@50 & zsR@100  \\
				\hline
				% VLK \cite{lu2016visual} & 8.45 & - & 3.36  & 3.75 & - & - & 3.13 & 3.52 & - & -   \\
				% VTransE \cite{zhang2017visual} & - & -  & 2.65  & 3.51 & - & - &  1.71 & 2.14 & - & -   \\
				
				IMP & CE-Loss &  12.17 & 17.66 & - & 2.09& 3.3 &- & 0.14& 0.39  & -\\ 
				IMP & Ours & &  &  &  &  &  &  &  &  \\ \hline
				
				Motif & CE-Loss & 5.79  &	11.02	& 14.74 & 1.06	& 2.18 &	3.07 & 0.02	& 0.08	& 0.24\\ 
				Motif & Ours & &  &  &  &  &  &  &  &  \\ \hline
				
    			Motif-TDE & CE-Loss & 8.28&	14.31	&18.04& 1.91	&2.95&	4.10& 1.54	&2.33	&3.03 \\ 
				Motif-TDE & Ours & 9.33 & 14.43 & 17.21 & 1.87 & 2.99 & 3.76 & 2.06 & 3.05 & 3.72 \\ \hline
				
				VCTree & CE-Loss & 1.43 & 4 & -& 0.39& 1.2 & - & 0.19& 0.46 & - \\ 
			    VCTree & Ours, LIN only & 5.35 & 10.51 & 14.18 &  &  &  &  &  &  \\ 
				VCTree & Ours, LIN+Mixup+KL &  & &  &  &  &  &  &  &  \\ 
				VCTree & Ours, LIN+Mixup-Allsamples+KL & &  &  &  &  &  &  &  &  \\ \hline
			
				VCTree & EBM-Loss & 2.25 & 5.36 & - & 0.87& 1.87 & - & 0.21& 0.54& -     \\ 
				VCTree & Ours, LIN only & 1.72 & 3.86 & 5.12 &  &  &  &  &  &  \\
				VCTree & Ours, LIN+Mixup+KL & 1.41 & 2.59 & 3.56 &  &  &  &  &  &  \\ 
				VCTree & Ours, LIN+Mixup-Allsamples+KL & 1.06 &1.68 & 2.36 & 0.70 & 1.51 & 1.86 &  &  &  \\ \hline
			
				VCTree-TDE & CE-Loss & 8.98 & 14.52 & - & 3.16 & 4.97 & - & 1.47 & 2.3 & - \\ 
				% VCTree-TDE & EBM-Loss & 9.58 & 15.14 & - & 4.18 & 6.38 & - & 1.62 & 2.68 & - \\ 
				VCTree-TDE & Ours, LIN only  & 8.56 & 13.54 & 17.36 &  &  &  &  &  &  \\ 
				VCTree-TDE & Ours & &  &   &  &  &  &  &  &  \\ \hline\hline

				\hline

\end{tabular}}
\caption{SOTA on Zero Shot Recall:Visual Genome dataset.}
\label{table:zeroshotvrd}
\end{table*}

\section{Statistcs}

\begin{figure*}
\begin{center}
\includegraphics[width=0.9\linewidth]{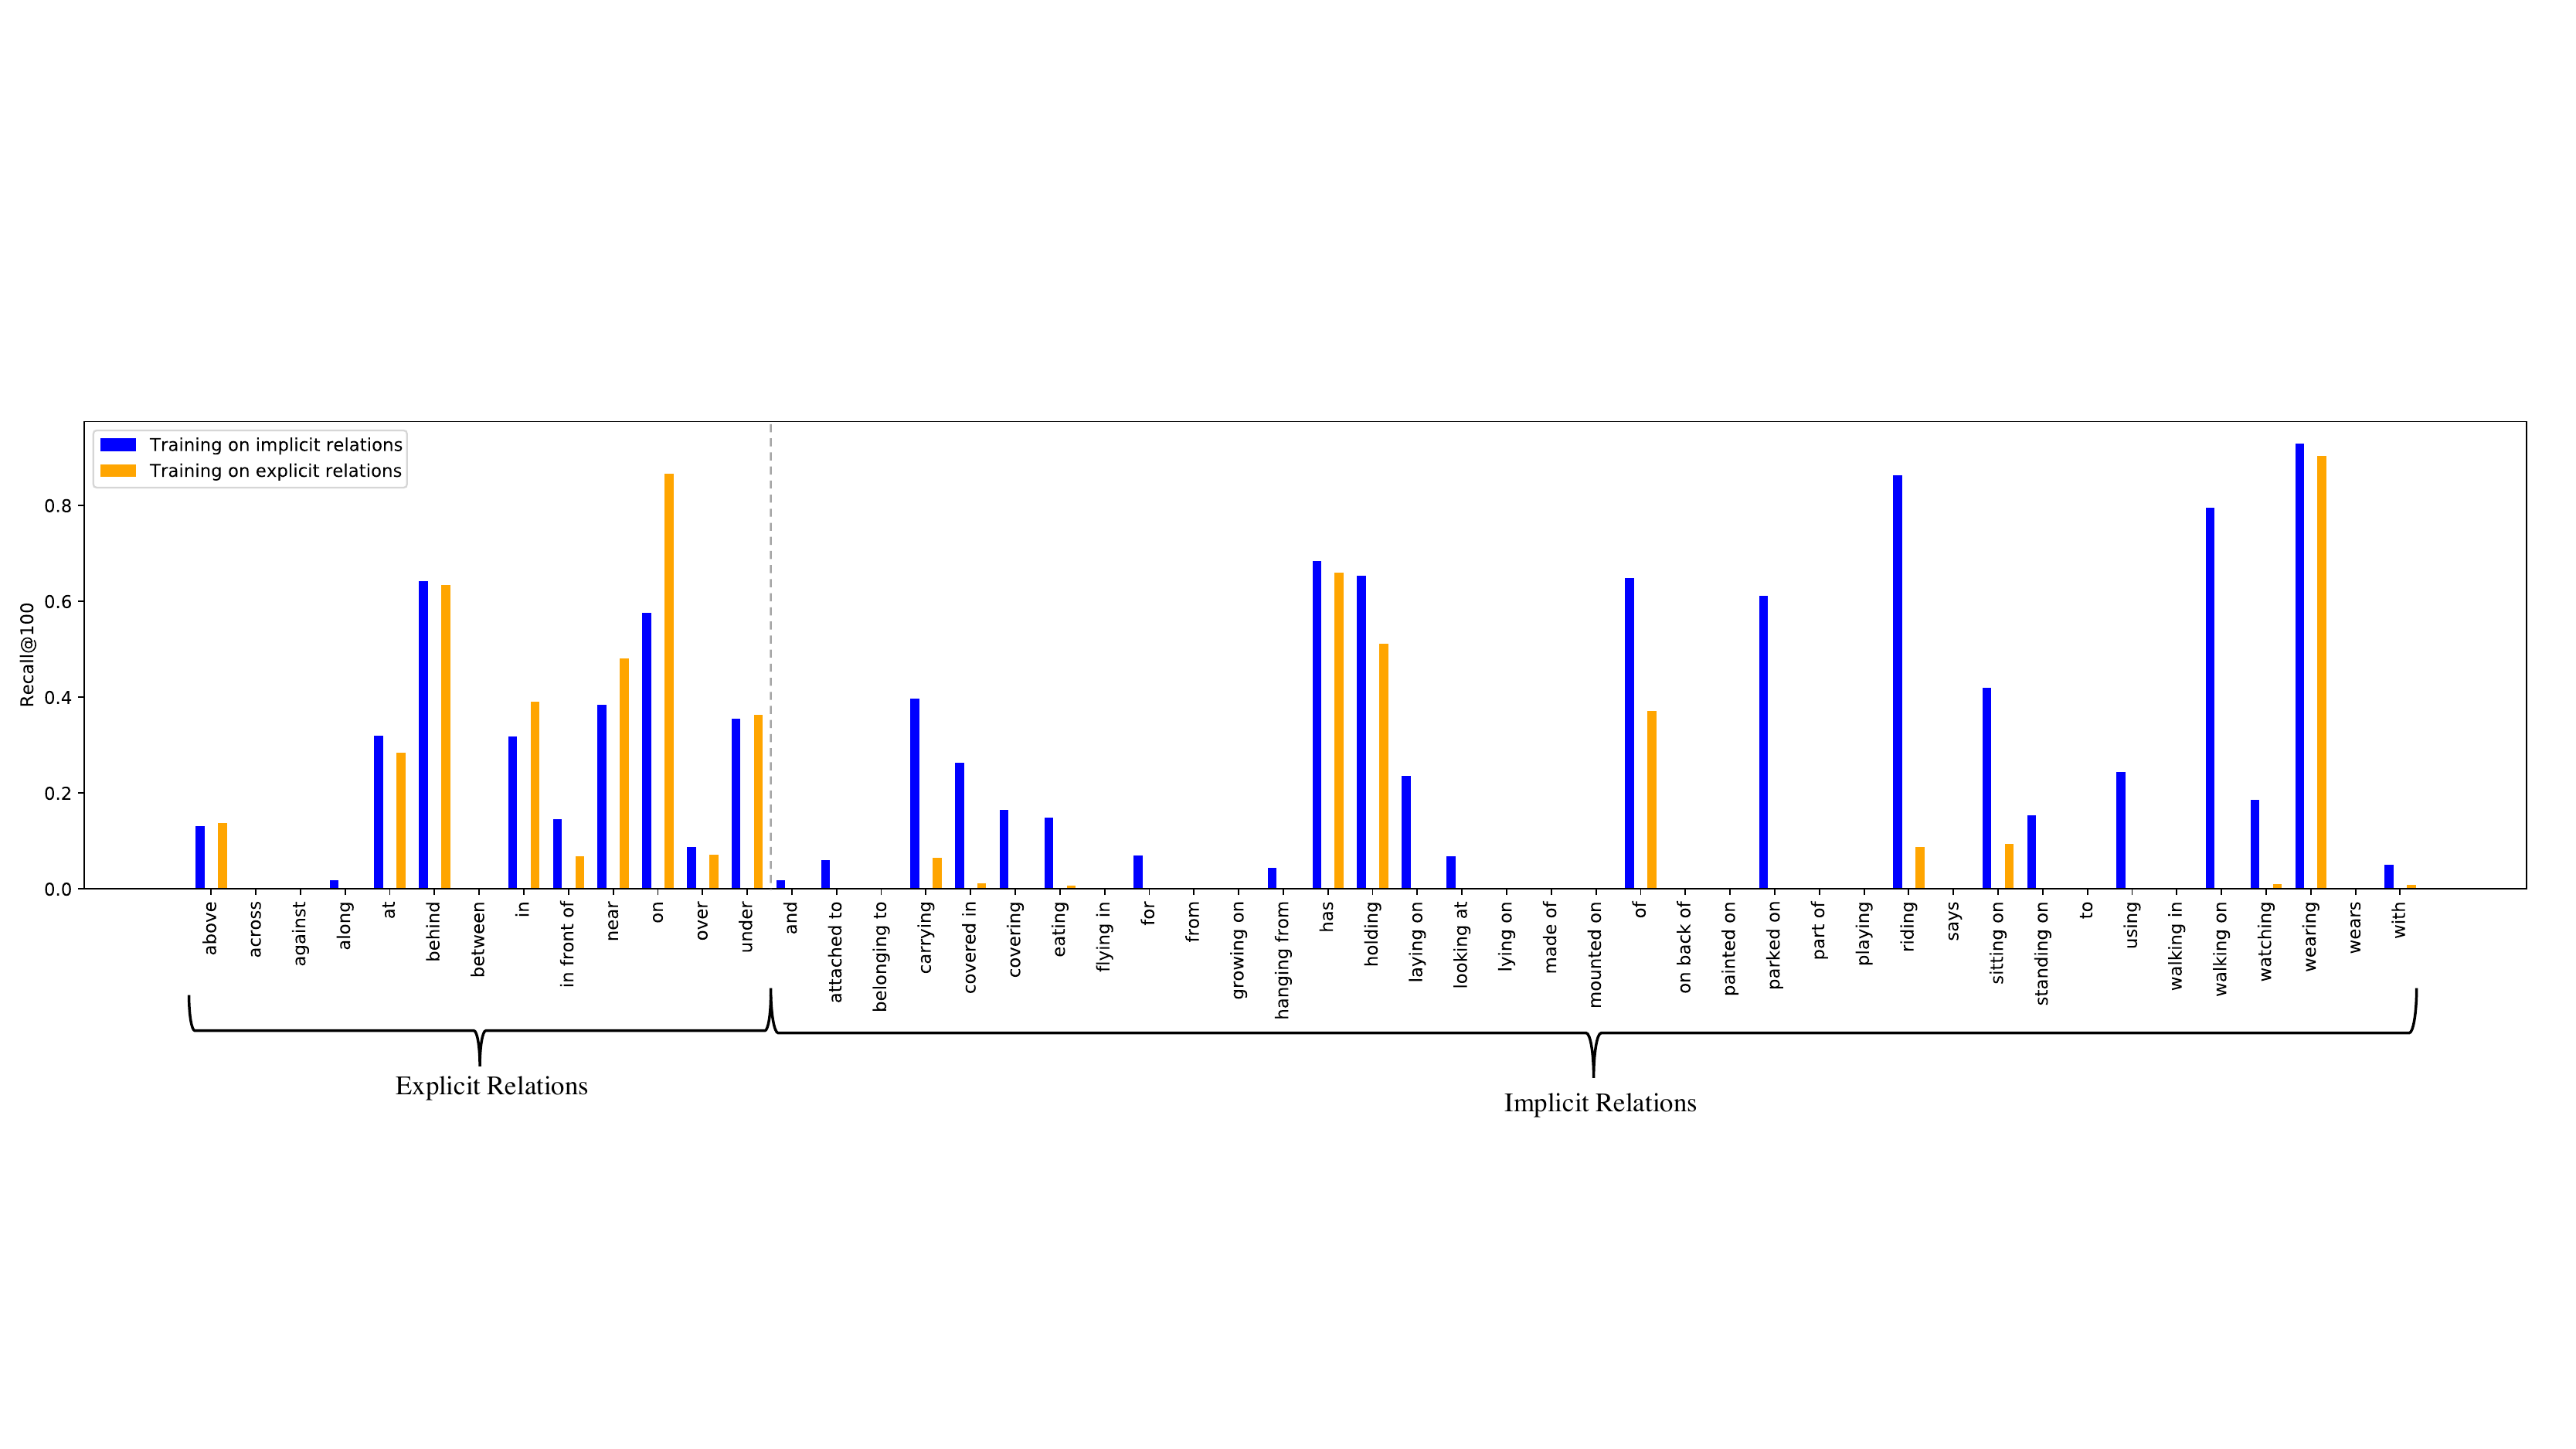}
% \vspace{-.3cm}
\end{center}
\caption{ }
\label{fig:imp_exp}
\end{figure*}
